# Supplementary material for: Hand-Object Interaction Controller (HOIC): Deep Reinforcement Learning for Reconstructing Interactions with Physics
Source: arXiv:2405.02676 source file (2024-05-04)
Supplement: Supplementary file 1 [file supp.tex]

\section{Implementation Details}

\subsection{Imitation Policy}
We follow a standard Actor-Critic framework \cite{sutton1998introduction} to design our imitation policy. 
The policy network and the value function network are both three-layer MLP with GeLU activation.
The output of the policy is the mean of a Gaussian distribution for the action, with the variance of the distribution being a fixed value $\sigma^2$.
During training, actions are sampled from the distribution, while during inference, actions are determined using the mean.
We use PPO \cite{schulman2017proximal} and Adam optimizer to train the policy and value function networks.
At each training epoch, a batch of $n=50000$ samples is collected.
Using these samples, multi-step returns are calculated through the TD($\lambda$) algorithm \cite{sutton1998introduction} and used for training the value network, and advantages are computed through the GAE($\lambda$) \cite{schulman2015high} to train the policy network.
All the parameters for training are shown in Tab.~\ref{tab:train_param}.

\begin{table}[H]
\caption{Parameters for training the imitation policy.}
\label{tab:train_param}
\begin{tabular}{lc}
\toprule
\textbf{Parameter}       & \textbf{Value}                 \\
\midrule
Policy MLP Layers    & {[}2048, 1024, 512{]} \\
Value MLP Layers     & {[}2048, 1024, 512{]} \\
Discount Factor $\gamma$      & 0.95                  \\
$\lambda$ for TD and GAE       & 0.95                  \\
Policy Learning Rate & $5.0 \times 10^{-5}$                 \\
Value Learning Rate  & $3.0 \times 10^{-4}$                 \\
PPO Clip Ratio $\epsilon$      & 0.2                   \\
Batch Size $n$          & 50000                 \\
Std $\sigma$             & 0.1                  \\
\bottomrule
\end{tabular}
\end{table}

\subsection{Reward Function}
The weights of the reward function are shown in Tab.~\ref{tab:w_reward}

% \begin{table*}[]
% \caption{Weights of the reward function.}
% \label{tab:w_reward}
% \begin{tabular}{lcccccccc}
% \textbf{Parameter} & $w^{\text{pose}}$ & wjoint & worient & wvel & wotrans & worot & wovel & wtorque \\
% \textbf{Value}     & 0.25  & 0.45   & 0.2     & 0.1  & 0.3     & 0.6   & 0.1   & 1e4     \\
% \textbf{Parameter} & kpose & kjoint & korient & kvel & kotrans & korot & kovel & kres    \\
% \textbf{Value}     & 6.0   & 12.0   & 3.0     & 0.05 & 10.0    & 1.0   & 0.05  & 1.0    
% \end{tabular}
% \end{table*}

\begin{table}[]
\caption{Weights of the reward function.}
\label{tab:w_reward}
\begin{tabular}{lcclc}
\toprule
\multicolumn{1}{l}{\textbf{Parameter}} & \multicolumn{1}{l}{\textbf{Value}} &\quad\quad &\multicolumn{1}{l}{\textbf{Parameter}} & \multicolumn{1}{l}{\textbf{Value}} \\
\midrule
$w^{\text{pose}}$                                  & 0.25              &\quad\quad                 & $k^{\text{pose}}$                                    & 6.0                                \\
$w^{\text{joint}}$                                 & 0.45              &\quad\quad                 & $k^{\text{joint}}$                                 & 12.0                               \\
$w^{\text{orient}}$                                & 0.2               &\quad\quad                 & $k^{\text{orient}}$                                & 3.0                                \\
$w^{\text{vel}}$                                     & 0.1               &\quad\quad                 & $k^{\text{vel}}$                                   & 0.05                               \\
$w^{\text{opose}}$                                & 0.9               &\quad\quad                 & $k^{\text{otrans}}$                                & 1.0                               \\
$w^{\text{ovel}}$                                    & 0.1               &\quad\quad                 & $k^{\text{ovel}}$                                  & 0.05                               \\
$w^{\text{torque}}$                                  & 100               &\quad\quad                 & $k^{\text{phys}}$                                   & 1.0                               \\
\bottomrule
\end{tabular}
\end{table}

\subsection{Training Strategies}
Following \cite{peng2018deepmimic}, we apply random start and early stop strategies in our sampling period.  
To collect samples, we randomly select a motion sequence from the dataset as the reference each time, and then randomly choose a frame from the motion as the initial state and start imitating.
The imitation will be early terminated when the imitation result differs significantly from the reference.
The judgment criteria for the difference are that the average joint error of the hand is greater than $10cm$, the object position error is greater than $10cm$, or the object rotation error is greater than $1rad$.
